# Supplementary material for: Content and Colour Distillation for Learning Image Translations with the Spatial Profile Loss
Source: arXiv:1908.00274 source file (2019-08-01)
Supplement: Supplementary file 1 [file supplementary.tex]

\newpage
\section*{Supplementary Material}

\setcounter{section}{0}
\section{Image-to-Image Domain Mapping}

\\ \\
\textbf{Cityscapes Evaluation:} We trained the FCN8 model~\cite{long2015fully} on the Cityscapes training set on a resolution of $256\times512$ using a Tensorflow~\cite{tensorflow} implementation. We use an adaptive learning rate starting with $10^{-4}$  for the first 10000 iterations decaying down to $10^{-6}$ after 40000 and a batch size of 4. Please note that in the main paper Table 1 the FCN scores, class IOU and per pixel-accuracy, are always provided on the full cityscapes validation set. 
\\ \\
\noindent\textbf{$\mathbf{Thermal\rightarrow{Visible}}$ Face Translation:} Thermal-visible face mapping is a relatively recently emerging image translation problem. For its practical applications in law-enforcement, it is needed to develop methods that works for night-time surveillance. Due to its large modality gap, it is very difficult to match a face captured using the passive thermal sensors (mid-wave IR or Long-wave IR) with its visible photograph in the usual mugshot databases. Apart from the automated face recognition applications, it is very difficult to identify a given person in the thermal image for a human observer as well. GAN based image synthesis has recently shown promising results in synthesizing a visible domain image from its thermal input~\cite{zhang2017generative, zhang2018tv}. While learning a straight mapping via a typical GAN setup (e.g., pix2pix) seems plausible, in practice it suffers from identity switches. All recent GAN based thermal-visible face mapping approaches employ additional losses/ or networks e.g., based on perceptual loss and identity loss to specifically handle these identity switches. In contrast to these GAN approaches, we train a standard single generator network without any additional identity preserving setup. This is possible because of the control we have in our loss components and we can use these to our advantage. On this problem we simply add our GP loss (weighted) computed between generator output and the thermal input to the full objective $\mathcal{L}_{SPL}$ which is defined between output and the visible target. \begin{center}
$ \mathcal{L}(x,y)= \alpha \cdot GP(G(x;\theta),x) + \mathcal{L}_{SPL} $    
\end{center}
where $\alpha$ is set to $0.3$. This way our network learns to map the thermal to visible while trying to preserve the input shape. As our results depict, Figure 4 (in the main paper) as well as few more in Figure~\ref{fig:thermal_Output} here, it learns a plausible mapping while keeping the input identity intact. Although because of this we still see some artifacts around the cheek and nose regions, we show some examples of such artifacts in Figure~\ref{fig:thermal_Output} . The training is standard with batch size of $16$ using Carl dataset~\cite{espinosa2013new}. The Carls dataset has a total of  $4920 $ thermal and visible images of $41$ subjects. We use the training set of $1260$ thermal and visible pairs (total $2520$ images of $21$ subjects), as used in  \cite{sarfraz2017deep}, and the rest $1200$ pairs (total $2400$ images) of the remaining 20 subjects are used for test. The model is trained on provided single channel images for 50 epochs. 

\begin{figure*}[t]
\centering
  \begin{tabular}{cc}
      \includegraphics[width=0.45\linewidth]{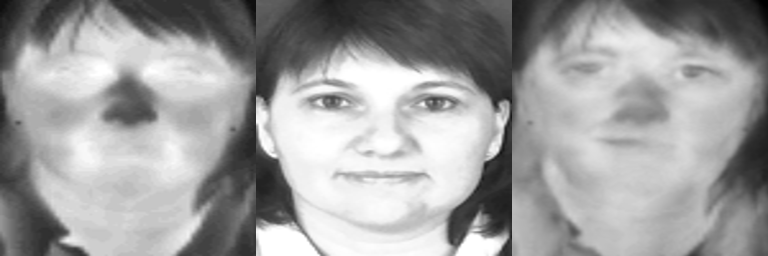}&
      \includegraphics[width=0.45\linewidth]{images/thermal/20-1196.png}\\
      \begin{overpic}[width=0.45\linewidth]{images/thermal/538.png}
      \put(11.5,-5){Input}\put(47,-5){GT}\put(78,-5){SPL}
      \end{overpic}&
      \begin{overpic}[width=0.45\linewidth]{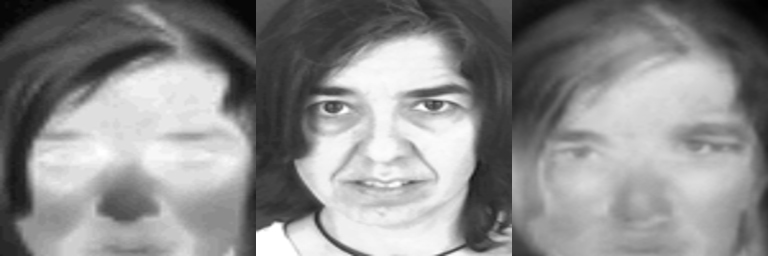}
      \put(11.5,-5){Input}\put(47,-5){GT}\put(78,-5){SPL}
      \end{overpic}\\\\      
  \end{tabular}

\caption{Limitations of our SPL on $thermal~\rightarrow~visible$: On Four Test Subjects:- showing typical artefacts around nose and mouth regions and failure cases. From left to right: Input thermal, Target visible and our SPL output}
\label{fig:thermal_Output}
\end{figure*}

\section{Single Image Super Resolution}
\noindent\textbf{Training Details:} The network has been trained on 4 times unknown downscaled LR images from DIV2K track 2, by taking a random patch of $96\times96$ from the input images LR images and corresponding patch from HR targets. Both the LR-HR training images are normalized to the range $[-1,1]$. For training, we use Adam~\cite{Adam}, with a fixed learning rate of $2 \times 10^{-4}$ and $\beta = 0.9$. The network is trained from scratch for 50 epochs.

Figure~\ref{fig:SR-SPL_Output} shows full image, LR, high-res GT and the restored output of our SR-SPL on a validation image ('0877') from DIV2K track 2.
%Our model has produced realistic result having fine texture and structure details very similar to the actual ground truth.
Despite the presence of unknown blur and noise in the input LR image, the SR-SPL synthesis depicts the ability of our $\mathcal{L}_{SPL}$ loss to train an off-the-shelf SR generator and recover the underlying texture/colour and content/structure details. 

As also presented in the main paper (Figure 5), Figure \ref{fig:SR-SPL} presents a more detailed comparison of our SR-SPL with state-of-the-art supervised SISR methods: FSRCNN~\cite{FSRCNN}, EDSR~\cite{EDSR} and SRGAN~\cite{SRGAN} on the DIV2k track 2 validation set. Here we also include the fully restored SR results (For more details either zoom in or extract the images using a document viewer) from all the compared approaches in addition to the cropped patches. Note that, PSNR/SISM values, reported at the bottom of each individual image-patch pair, are the performance of respective model on the full resolution images and not just the cropped patches. From our results, it can be seen that our SR-SPL is able to restore the fine structural details where other models suffer smoothness and other artefacts. Consider the cropped patch of middle image ('0816'), where both SR-SPL and EDSR\textsuperscript{+} have almost similar PSNR value, however, our SR-SPL manages to restore the very fine sculpture pattern details with minimal smoothness as compared to the output of EDSR\textsuperscript{+}. 

\clearpage
\setlength{\abovecaptionskip}{2pt}
\setlength{\belowcaptionskip}{-10pt}
\begin{figure*}
\centering
  \begin{tabular}{c<{\hspace{-0.7pc}}c<{\hspace{-0.7pc}}c}
      \includegraphics[width=0.3\linewidth]{images/supplementary/hilo/0877x4_LR.png} &
      \includegraphics[width=0.3\linewidth]{images/supplementary/hilo/0877x4_GON_1.png}&
      \includegraphics[width=0.3\linewidth]{images/supplementary/hilo/0877x4_HR.png} \\
      LR Input & Our SR-SPL  & HR Ground Truth
  \end{tabular}

\caption{Result of our SR-SPL on '0877' image from validation set of DIV2K track 2 with unknown downscaling. The LR image with $288 \times 510$ resolution has been upscaled by a factor of 4, resulting in $1152 \times 2040$. Our SR-SPL has reproduced high quality SR image with fine details similar to the HR ground truth.}
\label{fig:SR-SPL_Output}
\end{figure*}

\let\oldincludegraphics\includegraphics
\newcommand{\scalefiginput}[2][1]{%
  % Update \includegraphics to scale its argument
  \renewcommand{\includegraphics}[2][]{\scalebox{#1}{\oldincludegraphics[##1]{##2}}}%
  \input{#2}% Input figure
  % Restore \includegraphics
  \let\includegraphics\oldincludegraphics
}

\begin{figure*}
\centering

\begin{tabular}{c<{\hspace{-0.925pc}}c<{\hspace{-0.925pc}}c<{\hspace{-0.925pc}}c<{\hspace{-0.925pc}}c}
     \includegraphics[width=0.185\linewidth]{images/HiLo/gt_0801.png}
     & \includegraphics[width=0.185\linewidth]{images/HiLo/bicubic_0801.png}
     & \includegraphics[width=0.185\linewidth]{images/HiLo/EDSR+_0801.png}
     & \includegraphics[width=0.185\linewidth]{images/HiLo/SRGAN+_0801.png}
     %& \includegraphics[width=0.16\linewidth]{images/HiLo/CinCGAN_0801.png}
     & \includegraphics[width=0.185\linewidth]{images/HiLo/GON_0801.png}
     \\\includegraphics[width=0.185\linewidth]{images/HiLo/gt_0801_cropped.png}
     & \includegraphics[width=0.185\linewidth]{images/HiLo/bicubic_0801_cropped.png}
     & \includegraphics[width=0.185\linewidth]{images/HiLo/EDSR+_0801_cropped.png}
     & \includegraphics[width=0.185\linewidth]{images/HiLo/SRGAN+_0801_cropped.png}
     %& \includegraphics[width=0.16\linewidth]{images/HiLo/CinCGAN_0801_cropped.png}
     & \includegraphics[width=0.185\linewidth, height=0.1138\linewidth]{images/HiLo/GON_0801_cropped.png}
     \\\\ \footnotesize Ground Truth & \footnotesize Bicubic & \footnotesize EDSR\textsuperscript{+}~\cite{EDSR} & \footnotesize SRGAN\textsuperscript{+}~\cite{SRGAN}
     %& CinCGAN~\cite{CinCGAN}
     &\footnotesize \textbf{SR-SPL (ours)} 
     \\\\ \footnotesize PSNR/SSIM & 23.22/0.64 & 26.23/0.68 & 24.06/0.58
    % & 24.83/0.65
     & 27.71/0.80
     \\\\\includegraphics[width=0.185\linewidth]{images/HiLo/gt_0816.png}
     & \includegraphics[width=0.185\linewidth]{images/HiLo/bicubic_0816.png}
     & \includegraphics[width=0.185\linewidth]{images/HiLo/EDSR+_0816.png}
     & \includegraphics[width=0.185\linewidth]{images/HiLo/SRGAN+_0816.png}
    % & \includegraphics[width=0.16\linewidth]{images/HiLo/CinCGAN_0816.png}
     & \includegraphics[width=0.185\linewidth]{images/HiLo/GON_0816.png}
     \\\includegraphics[width=0.185\linewidth]{images/HiLo/gt_0816_a.png}
 & \includegraphics[width=0.185\linewidth]{images/HiLo/bicubic_0816_a.png}
     & \includegraphics[width=0.185\linewidth]{images/HiLo/EDSR+_0816_a.png}
     & \includegraphics[width=0.185\linewidth]{images/HiLo/SRGAN+_0816_a.png}
    % & \includegraphics[width=0.16\linewidth]{images/HiLo/CinCGAN_0816_a.png}
     & \includegraphics[width=0.185\linewidth, height=0.11882\linewidth]{images/HiLo/GON_0816_a.png}
     \\\includegraphics[width=0.185\linewidth]{images/HiLo/gt_0816_b.png}
     & \includegraphics[width=0.185\linewidth]{images/HiLo/bicubic_0816_b.png}
     & \includegraphics[width=0.185\linewidth]{images/HiLo/EDSR+_0816_b.png}
     & \includegraphics[width=0.185\linewidth]{images/HiLo/SRGAN+_0816_b.png}
     %& \includegraphics[width=0.16\linewidth]{images/HiLo/CinCGAN_0816_b.png}
     & \includegraphics[width=0.185\linewidth,height=0.05146\linewidth]{images/HiLo/GON_0816_b.png}
     \\\\ Ground Truth & Bicubic & EDSR\textsuperscript{+}~\cite{EDSR} & SRGAN\textsuperscript{+}~\cite{SRGAN}
     %& CinCGAN~\cite{CinCGAN}
     & \textbf{SR-SPL (ours)}
     \\\\ PSNR/SSIM & 22.25/0.68 &  29.06/0.75 & 27.36/0.68
     %& 27.95/0.72
     & 29.11/0.81
     \\\\\includegraphics[width=0.185\linewidth]{images/HiLo/gt_0853.png}
     & \includegraphics[width=0.185\linewidth]{images/HiLo/bicubic_0853.png}
     & \includegraphics[width=0.185\linewidth]{images/HiLo/EDSR+_0853.png}
     & \includegraphics[width=0.185\linewidth]{images/HiLo/SRGAN+_0853.png}
     %& \includegraphics[width=0.16\linewidth]{images/HiLo/CinCGAN_0853.png}
     & \includegraphics[width=0.185\linewidth]{images/HiLo/GON_0853.png}
     \\\includegraphics[width=0.185\linewidth]{images/HiLo/gt_0853_cropped.png}
     & \includegraphics[width=0.185\linewidth]{images/HiLo/bicubic_0853_cropped.png}
     & \includegraphics[width=0.185\linewidth]{images/HiLo/EDSR+_0853_cropped.png}
     & \includegraphics[width=0.185\linewidth]{images/HiLo/SRGAN+_0853_cropped.png}
    % & \includegraphics[width=0.16\linewidth]{images/HiLo/CinCGAN_0853_cropped.png}
     & \includegraphics[width=0.185\linewidth, height=0.1247\linewidth]{images/HiLo/GON_0853_cropped.png}
     \\\\  \footnotesize Ground Truth &  \footnotesize Bicubic &  \footnotesize EDSR\textsuperscript{+}~\cite{EDSR} &  \footnotesize SRGAN\textsuperscript{+}~\cite{SRGAN}
     %& CinCGAN~\cite{CinCGAN} 
     &  \footnotesize \textbf{SR-SPL (ours)} 
     \\\\ \footnotesize  PSNR/SSIM & 26.81/0.83 &  30.28/0.88 & 29.05/0.85
     %&  28.26/0.84 
     & 29.60/0.87
     
\end{tabular}
\caption{Super-resolution results of '0801', '0816' and '0853' (DIV2K) with scale factor ×4. EDSR\textsuperscript{+} and SRGAN\textsuperscript{+} are trained on paired DIV2K track 2 dataset~\cite{CinCGAN}. SR-SPL (ours) achieves the state-of-the-art and restore sharper details.}
\label{fig:SR-SPL}
\end{figure*}

\setlength{\abovecaptionskip}{5pt}
\setlength{\belowcaptionskip}{1pt}
\clearpage

\section{Photo-realistic Makeup Transfer}
\noindent\textbf{FCC Dataset:}
In Figure \ref{fig:dataset}, we provide sample images of the FCC database for the three categories: Strongly visible makeup, mildly visible makeup and no makeup. The face images contain varying poses, lighting and race.

\begin{figure*}
\centering

\begin{tabular}{c<{\hspace{-0.8pc}}c<{\hspace{-0.8pc}}c<{\hspace{-0.8pc}}c<{\hspace{-0.8pc}}c<{\hspace{-0.8pc}}c}
\includegraphics[width=0.16\linewidth]{images/dataset/dataset_M/2VyCTGWienU_00001_256_cropped.jpg}
 & \includegraphics[width=0.16\linewidth]{images/dataset/dataset_M/W2rMu4CgqLo_eof_00015_512_cropped.jpg}
 &\includegraphics[width=0.16\linewidth]{images/dataset/dataset_M/b2Yq0NIutjI_eof_00050_256_cropped.jpg}
 & \includegraphics[width=0.16\linewidth]{images/dataset/dataset_M/WxZPMJvJbkc_00040_256_cropped.jpg}
 & \includegraphics[width=0.16\linewidth]{images/dataset/dataset_M/P5OKiy5Rr0U_00191_512_cropped.jpg}
 & \includegraphics[width=0.16\linewidth]{images/dataset/dataset_M/5hTitrpK-v0_00052_512_cropped.jpg}

\end{tabular}
\vspace{0.75pt}
\hline
\vspace{2pt}
\begin{tabular}{c<{\hspace{-0.8pc}}c<{\hspace{-0.8pc}}c<{\hspace{-0.8pc}}c<{\hspace{-0.8pc}}c<{\hspace{-0.8pc}}c}
\includegraphics[width=0.16\linewidth]{images/dataset/dataset_medium/6yFB2TBxwwA_00046_512_cropped.jpg}
 & \includegraphics[width=0.16\linewidth]{images/dataset/dataset_medium/GAqWGv0W-TA_eof_00163_512_cropped.jpg}
 &\includegraphics[width=0.16\linewidth]{images/dataset/dataset_medium/0VGNwadgJ6k_eof_00041_512_cropped.jpg}
 & \includegraphics[width=0.16\linewidth]{images/dataset/dataset_medium/AuFST6yTzwk_eof_00096_512_cropped.jpg}
 & \includegraphics[width=0.16\linewidth]{images/dataset/dataset_medium/HH8xDoIWAp8_eof_00101_512_cropped.jpg}
 & \includegraphics[width=0.16\linewidth]{images/dataset/dataset_medium/BqkO9M7NZas_eof_00117_512_cropped.jpg}

\end{tabular}
\vspace{0.75pt}
\hline
\vspace{2pt}
\begin{tabular}{c<{\hspace{-0.8pc}}c<{\hspace{-0.8pc}}c<{\hspace{-0.8pc}}c<{\hspace{-0.8pc}}c<{\hspace{-0.8pc}}c}
\includegraphics[width=0.16\linewidth]{images/dataset/Dataset_NM/FjzwpwQqh9A_00138_256_cropped.jpg}
 & \includegraphics[width=0.16\linewidth]{images/dataset/Dataset_NM/_6dB_BJ6wiE_00059_256_cropped.jpg}
 &\includegraphics[width=0.16\linewidth]{images/dataset/Dataset_NM/0f9hFLmTvnU_00184_256_cropped.jpg}
 & \includegraphics[width=0.16\linewidth]{images/dataset/Dataset_NM/0L2zNXpBP3k_00027_256_cropped.jpg}
 & \includegraphics[width=0.16\linewidth]{images/dataset/Dataset_NM/BqkO9M7NZas_00137_512_cropped.jpg}
 & \includegraphics[width=0.16\linewidth]{images/dataset/Dataset_NM/Nj8NeLUeoiQ_00048_512_cropped.jpg}

\end{tabular}
\caption{Sample images from our proposed FCC dataset a.) strong makeup (top row), b.) less noticeable makeup (middle row)and c.) no makeup(bottom row). 
%\saquib{Constantin, 1st row 2nd image form left, and 2nd row last image (use at reference) and bottom row (last image as source) to show as an example of both our resnet and SR-SPL makeup transfer ??}
}
\label{fig:dataset}
\end{figure*}

\noindent\textbf{Training details Makeup SR-SPL:}
We train the SR-SPL for $4\times$ upscaling on our FCC database ($512 \times 512$ subset) for strongly visible makeup. We use the same proposed Makeup transfer sequence as explained in the Figure 6 of the main paper.  We resized (bicubically) the reference and source to $128 \times 128$, to make our $6$-channel LR input.
The original $\times4$ ($512 \times 512$) reference is used (to add at the output in our design) and as the target in the $\mathcal{L}_{SPL}$ loss optimization. After training for 10 epochs, since the SR-SPL generator is fully convolutional, we can generate a full HD $2048 \times 2048$ photo realistic portrait image of the source, with transferred reference makeup, from its LR $512 \times 512$ source and reference.
During test time the references are resized (bicubically) to match the generator output for adding them.

%As usually for single-image super-resolution, there exists no high resolution reference to add to the generator output. Therefore, we upscale the reference bicubically and add it to our intermediate output to maintain our makeup transfer sequence.\\

\noindent\textbf{More Qualitative Makeup Transfer Examples:}
As discussed in the main paper, we have trained two different generator architectures on this problem with our $\mathcal{L}_{SPL}$ objective. (1) The 9-block resnet generator used in pix2pix/cyclegan frameworks~\cite{pix2pix,cyclegan}, trained on $256 \times 256$ images, we term  SPL. (2) The super-resolution SRResNet generator~\cite{SRGAN} (SR-SPL). 
%In Figure \ref{fig:4} and \ref{fig:5}, we compare the results of SPL and SR-SPL on a mildy and a strongly visible makeup sample from our FCC test set. 

Similar to Figures 8 and 9 of the main paper, where we took input and reference from Chang~\etal\cite{chang2018pairedcyclegan}, we use input and references in Figure \ref{fig:6} from He~\etal\cite{he2017neural}. Here, we compare with Tong~\etal\cite{tong} and He~\etal\cite{he2017neural} as similar to us these methods also view the makeup transfer problem from a colour transfer perspective. Tong~\etal\cite{tong} do not quite solve the same problem of transferring makeup presented in a reference onto an input image as they make use of before- and after-images of the reference. He~\etal\cite{he2017neural} similar to Liao~\etal\cite{liao2017visual} solve an optimization problem using an assisting VGG-network.

\hspace{-10pt}
\begin{figure*}[pt]
\centering
\begin{tabular}{c<{\hspace{-0.6pc}}c<{\hspace{-0.6pc}}c<{\hspace{-0.6pc}}c<{\hspace{-0.6pc}}c<{\hspace{-0.6pc}}c}
\includegraphics[width=0.14\linewidth]{images/supplementary/nomakeup/2.png}
 & \includegraphics[width=0.14\linewidth]{images/supplementary/makeup/1.png}
 & \includegraphics[width=0.14\linewidth]{images/supplementary/tong/2.png}
 & \includegraphics[width=0.14\linewidth]{images/supplementary/he/2.png}
 &\includegraphics[width=0.14\linewidth]{images/supplementary/normal/21.png}
 & \includegraphics[width=0.14\linewidth]{images/supplementary/highres/21.png}
\\
Input & Reference&Tong~\etal\cite{tong} & He~\etal\cite{he2017neural} &SPL & SR-SPL
\end{tabular}
\caption{Comparison of Tong~\etal\cite{tong}, He~\etal\cite{he2017neural},SPL and SR-SPL.}
\label{fig:6}
\end{figure*}

\noindent \textbf{Makeup Transfer Limitations:} We show limitations of our approach in Figure \ref{fig:8} and \ref{fig:9}.  Case 1 in Figure \ref{fig:8} involves an input image with facial irregularities such as acne. Due to maintaining the overall facial structure of the input image SPL as well as SR-SPL cannot remove unwanted facial features (such as acne) when transferring the reference makeup. 
Case 2 in Figure \ref{fig:9} covers incorrectly warped references. When landmarks of either input or reference are wrongly estimated the warped reference  will lead to problems such as included background or not properly aligned faces. While our approach can  handle slight deviations, it cannot fully transfer seen makeup onto the resulting image in severe cases.

SPL and SR-SPL solve the makeup transfer problem for both cases of makeup. SPL shares stronger similarities to the source image, SR-SPL adopts more visual details of the reference. All SPL results are in a resolution of  $256\times256$, whereas our SR-SPL outputs are in $2048\times2048$.
%Both models can result into images appearing slightly darker than the source. 

For more details either zoom in or extract the images using a document viewer such as Evince. All of the results shown here and in the main paper are on the images which were never seen in the training. Especially, our Makeup comparison results are on the images taken/saved directly from the respective author's papers, these result shows a strong generalization ability of our trained SPL models.

\clearpage

\begin{figure*}[pt]
\centering
\begin{tabular}{c<{\hspace{-0.6pc}}c<{\hspace{-0.6pc}}c<{\hspace{-0.6pc}}c}
\includegraphics[width=0.225\linewidth]{images/supplementary/nomakeup/Nj8NeLUeoiQ_00048_512_cropped.jpg}
 & \includegraphics[width=0.225\linewidth]{images/dataset/dataset_medium/BqkO9M7NZas_eof_00117_512_cropped.jpg}
 & \includegraphics[width=0.225\linewidth]{images/supplementary/normal/Nj8NeLUeoiQ_00048_512_croppedNj8NeLUeoiQ_00048_512_croppedBqkO9M7NZas_eof_00117_512_cropped.jpg}
 & \includegraphics[width=0.225\linewidth]{images/supplementary/highres/Nj8NeLUeoiQ_00048_512_croppedNj8NeLUeoiQ_00048_512_croppedBqkO9M7NZas_eof_00117_512_cropped.jpg}
\\
Input & Reference &SPL & SR-SPL
\end{tabular}
\caption{Makeup transfer limitation: Case 1 for SPL and SR-SPL. Our method fails to fully remove potentially unwanted facial features such as acne.}
\label{fig:8}

\begin{tabular}{c<{\hspace{-0.6pc}}c<{\hspace{-0.6pc}}c<{\hspace{-0.6pc}}c}
\\\\
\includegraphics[width=0.225\linewidth]{images/supplementary/name/2normalhqdefault_in.jpg}
 & \includegraphics[width=0.225\linewidth]{images/supplementary/name/hqdefault3.jpg}
 & \includegraphics[width=0.225\linewidth]{images/supplementary/name/2normalhqdefault.jpg}
 & \includegraphics[width=0.225\linewidth]{images/supplementary/name/2normalhqdefault_out.jpg}
\\
Input & Reference & Warped &SPL\\
&&Reference&
\end{tabular}
\caption{Makeup transfer limitation: Case 2 for SPL and SR-SPL. Our method struggles when the reference is warped incorrectly.}
\label{fig:9}
\end{figure*}

\iffalse
\begin{figure*}[t]
\centering
\begin{tabular}{c<{\hspace{-0.8pc}}c<{\hspace{-0.8pc}}c<{\hspace{-0.8pc}}c<{\hspace{-0.8pc}}c<{\hspace{-0.8pc}}c}
\includegraphics[width=0.16\linewidth]{images/supplementary/nomakeup/src3ref3-4.png}
 & \includegraphics[width=0.16\linewidth]{images/supplementary/makeup/ref3-4.png}
 & \includegraphics[width=0.16\linewidth]{images/supplementary/chang/liuetal.png}
 & \includegraphics[width=0.16\linewidth]{images/supplementary/chang/liaoetal.png}
 &\includegraphics[width=0.16\linewidth]{images/supplementary/chang/pcganetal.png}
 & \includegraphics[width=0.16\linewidth]{images/supplementary/highres/sname.png}
\\
Input & Reference & Liu~\etal\cite{liu2016makeup}&Liao~\etal\cite{liao2017visual} & Chang~\etal\cite{chang2018pairedcyclegan}& SR-SPL
\end{tabular}
\caption{Comparison of Liu~\etal\cite{liu2016makeup}, Liao~\etal\cite{liao2017visual},  Chang~\etal\cite{chang2018pairedcyclegan} and SR-SPL. \constantin{I would consider leaing this one out, as we made 2 comparisons with chang in the main paper already, and in a way would argue that we just compare against the results of the people that we didnt compare with in the main paper.} \saquib{sure leave this out}} 
\label{fig:8}
\end{figure*}
\fi
